# Supplementary material for: Video-QTR: Query-Driven Temporal Reasoning Framework for Lightweight Video Understanding
Source: arXiv:2512.09354 source file (2025-12-10)
Supplement: Supplementary file 1 [file x_appendix.tex]

\section{Appendix}
\subsection{Abalation Study}
\label{app:aba}
\newcommand{\cmark}{\textcolor{green!60!black}{\checkmark}}
\newcommand{\xmark}{\textcolor{red!80!black}{\ding{55}}}

\begin{table*}[!t]
    \centering
    % --- 变更：Caption已更新，解释了新增的性能下降列 ---
    \caption{Ablation study of our proposed components on the Movie-Chat benchmark. We ablate three key components and report the absolute drop in Total Accuracy ('Acc. Drop \%') for each configuration relative to our full model, highlighting the contribution of each component.}
    \label{tab:ablation_moviechat_with_drop}
    \resizebox{\textwidth}{!}{%
    % --- 变更：表格总列数从10增加到11 (l ccc cc cc cc c) ---
    \begin{tabular}{l ccc cc cc cc c}
        \toprule
        \multirow{2}{*}{\textbf{Configuration}} & \textbf{Temporal} & \textbf{Conversational} & \textbf{Iterative Confidence} & \multicolumn{2}{c}{\textbf{Global Mode}} & \multicolumn{2}{c}{\textbf{Breakpoint Mode}} & \multicolumn{2}{c}{\textbf{Total}} & \textbf{Acc. Drop} \\
        \cmidrule(lr){2-4} \cmidrule(lr){5-6} \cmidrule(lr){7-8} \cmidrule(lr){9-10} \cmidrule(lr){11-11}
         & \textbf{Segment Selector} & \textbf{Memory} & \textbf{Refinement} & \textbf{Acc. (\%)} & \textbf{Score} & \textbf{Acc. (\%)} & \textbf{Score} & \textbf{Acc. (\%)} & \textbf{Score} & \textbf{(\%)} \\
        \midrule
        % --- 变更：multicolumn的跨列数改为11 ---
        \rowcolor{gray!20}
        \multicolumn{11}{c}{\textit{Ablation of individual components from our full model:}} \\
        % --- 变更：在每行末尾添加计算出的性能下降值 ---
        w/o RTP & \xmark & \cmark & \cmark & 69.44 & 3.49 & 40.98 & 2.06 & 47.55 & 2.38 & \textcolor{red!80!black}{30.40} \\
        w/o TM & \cmark & \xmark & \cmark & 79.70 & 3.98 & 67.17 & 3.36 & 71.60 & 3.58 & \textcolor{red!80!black}{6.35} \\
        w/o TCR & \cmark & \cmark & \xmark & 73.91 & 3.69 & 61.94 & 3.11 & 64.70 & 3.24 & \textcolor{red!80!black}{13.25} \\
        \midrule
        \textbf{Video-QTR (Full Model)} & \cmark & \cmark & \cmark & \textbf{88.72} & \textbf{4.45} & \textbf{74.72} & \textbf{3.60} & \textbf{77.95} & \textbf{3.94} & --- \\
        \bottomrule
    \end{tabular}%
    }
\end{table*}
